# Supplementary material for: Coding of 3D Videos Based on Visual Discomfort
Source: arXiv:1811.08821 ancillary file (2018-11-21)

## Coding of 3D Videos based on Visual Discomfort

Can Temel and Ghassan AlRegib  
School of Electrical and Computer Engineering  
Georgia Tech, Atlanta, GA

November 5, 2013

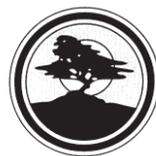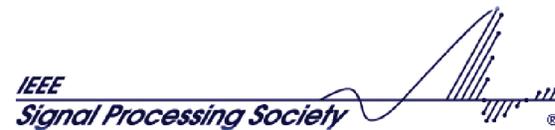

1. **3VQM: A 3D Video Quality Measure**
2. **3VQM versus VDM**
3. **VDM versus SSIM and PSNR**
4. **Encoding Mode Selection**
5. **Rate Distortion Analysis**
6. **Conclusion**

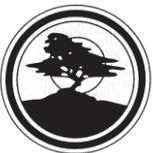

# A 3D Video Quality Measure (3VQM)

Stereoscopic 3D

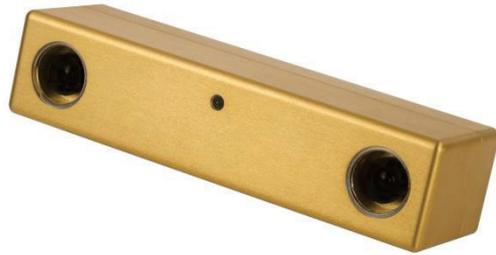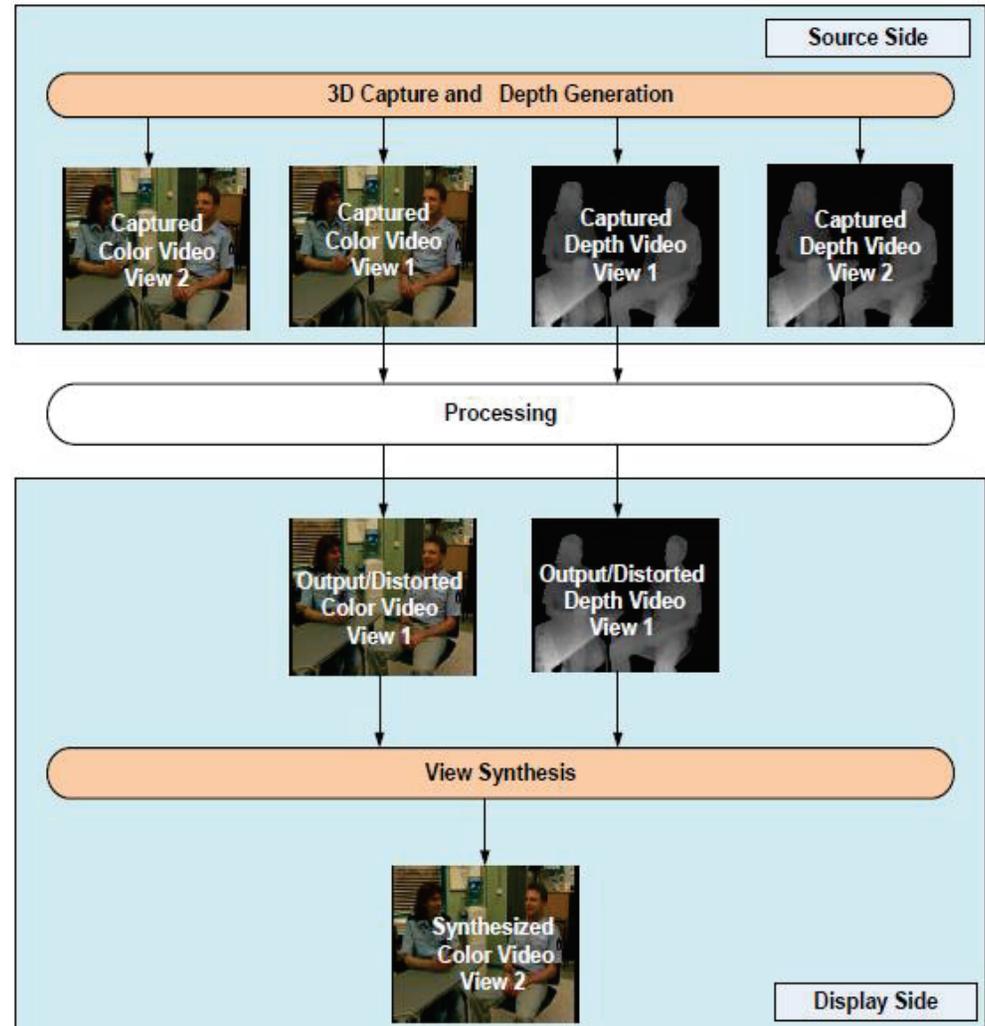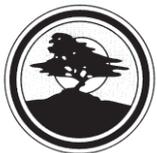

# A 3D Video Quality Measure (3VQM)

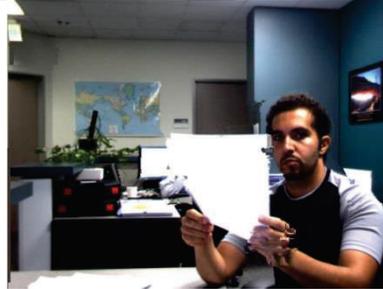

$$\Delta Z = |Z_{ideal} - Z|$$

**Spatial Outliers (SO)**  
 $STD(\Delta Z)$

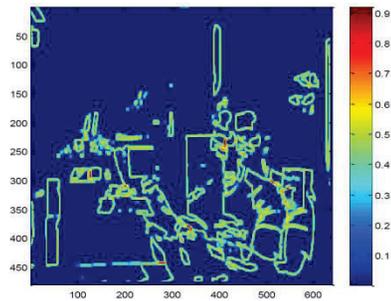

Standard deviation of depth map errors

**Temporal Outliers (TO)**  
 $STD(\Delta Z_K - \Delta Z_{K-1})$

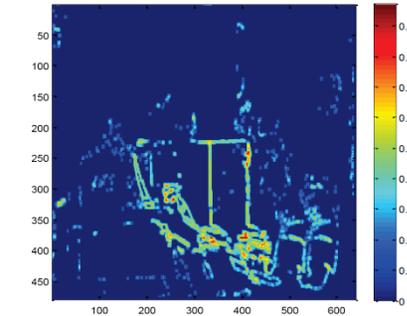

Standard deviation of two depth map errors in time domain

**Temporal Inconsistencies (TI)**  
 $STD(Z_K - Z_{K-1})$

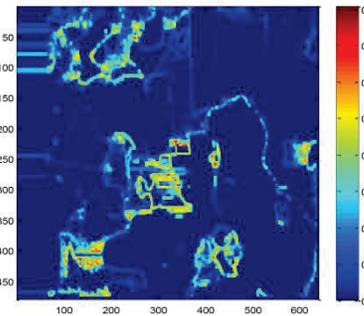

Standard deviation of two depth values in two time instances

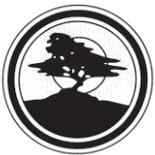

# A 3D Video Quality Measure (3VQM)

**RMSE:** Root Mean Squared Error

**CC:** Pearson Linear Correlation Coefficient

**ROCC:** Spearman Rank Order Correlation Coefficient

**MAE:** Mean Absolute Error

**Low RMSE:** Accuracy

**High CC:** Coherency

**High ROCC:** Coherency

**Low MAE:** Accuracy

|                       | RMSE        | CC          | ROCC        | MAE         |
|-----------------------|-------------|-------------|-------------|-------------|
| Average PSNR          | 0.95        | 0.73        | 0.72        | 0.82        |
| Weighted Average PSNR | 0.94        | 0.76        | 0.78        | 0.79        |
| Average SSIM          | 0.81        | 0.60        | 0.54        | 0.62        |
| <b>3VQM</b>           | <b>0.62</b> | <b>0.89</b> | <b>0.79</b> | <b>0.52</b> |

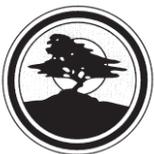

# A 3D Video Quality Measure (3VQM)

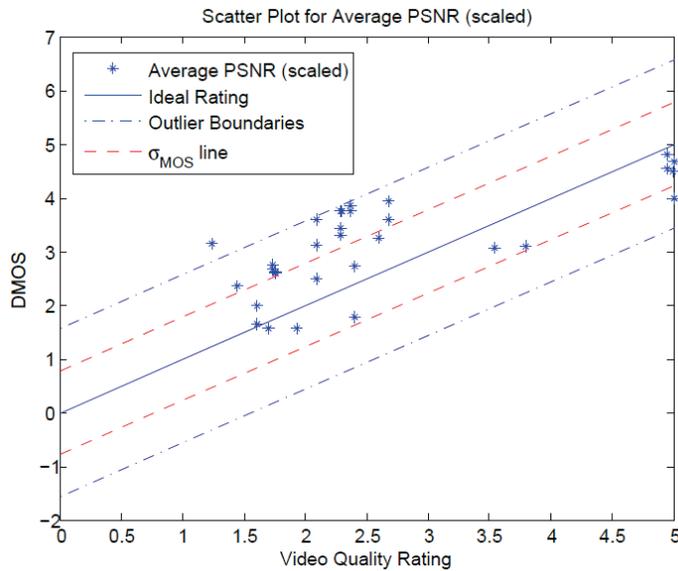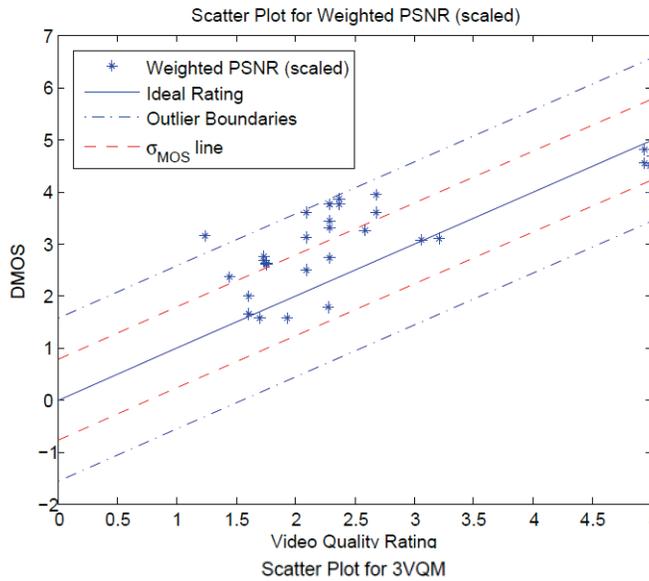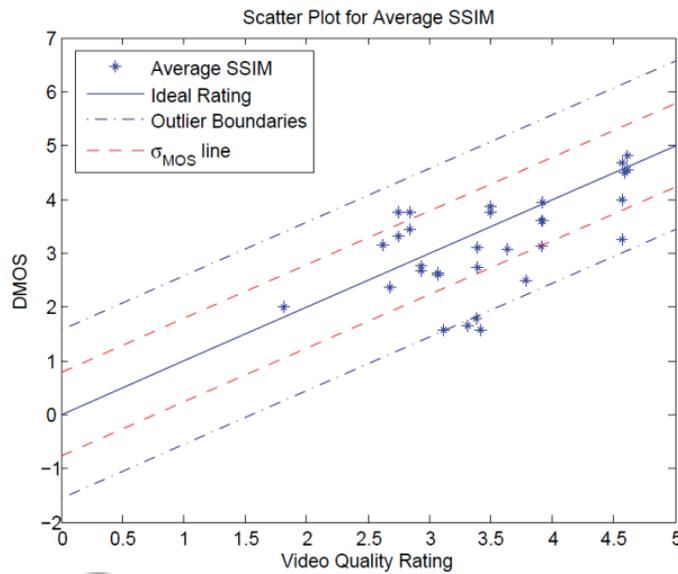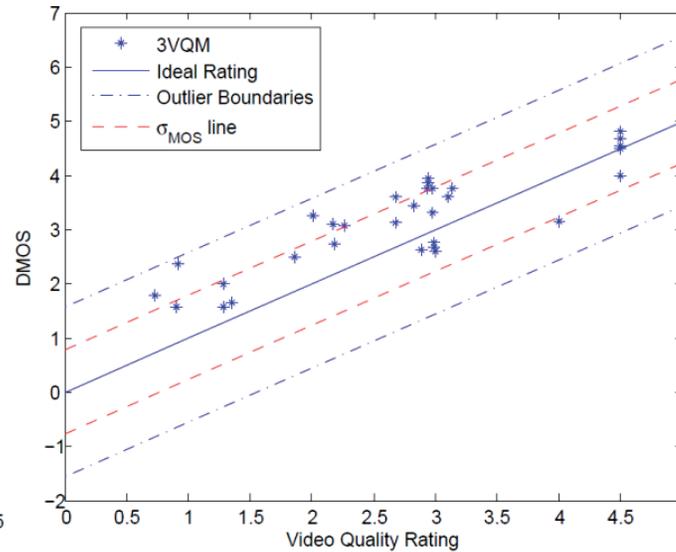

OR: Outlier Ratio Low OR: Consistency

|                       | OR          |
|-----------------------|-------------|
| Average PSNR          | 0.19        |
| Weighted Average PSNR | 0.19        |
| Average SSIM          | 0.13        |
| <b>3 VQM</b>          | <b>0.00</b> |

# 3VQM versus VDM

|                                 | 3VQM                                            | VDM                                              |
|---------------------------------|-------------------------------------------------|--------------------------------------------------|
| <b>Error</b>                    | $\Delta Z =   Z_{ideal} - Z_{GT}  $             | $\Delta \hat{Z} =   Z_{GT} - Z_{processed}  $    |
| <b>Spatial Outliers</b>         | STD( $\Delta Z$ )                               | STD( $\Delta \hat{Z}$ )                          |
| <b>Temporal Outliers</b>        | STD( $\Delta Z_{t+1} - \Delta Z_t$ )            | STD( $\Delta \hat{Z}_{t+1} - \Delta \hat{Z}_t$ ) |
| <b>Temporal Inconsistencies</b> | STD( $Z_{t+1} - Z_t$ )                          | STD( $\hat{Z}_{t+1} - \hat{Z}_t$ )               |
| <b>Fusing method</b>            | $K(1 - SO(SO \cap TO))^a (1 - TO)^b (1 - TI)^c$ | $K(1 - SO)^a (1 - TO)^b (1 - TI)^c$              |
| <b>K</b>                        | 5.0                                             | 1.0                                              |
| <b>a</b>                        | 8                                               | $\sqrt[3]{\text{Spatial Information Index}}$     |
| <b>b</b>                        | 8                                               | $\sqrt[3]{\text{Temporal Information Index}}$    |
| <b>c</b>                        | 6                                               | 0                                                |

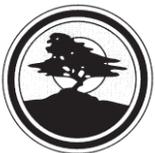

# 3VQM versus VDM

$$SInf = \sqrt[3]{\max_{time}\{std_{space}[Sobel(F_n)]\}} \quad M_n(i,j) = F_n(i,j) - F_{n-1}(i,j) \quad TInf = \sqrt[3]{\max_{time}\{std_{space}[M_n(i,j)]\}}$$

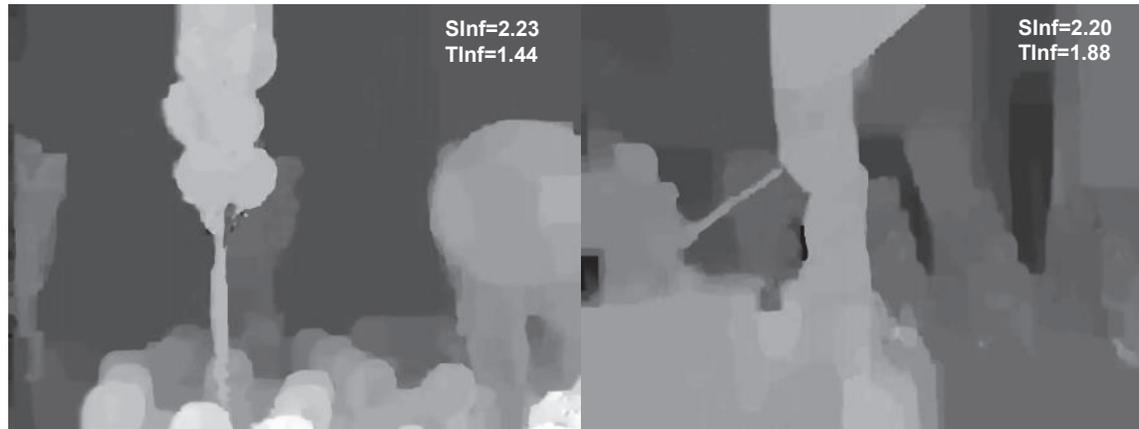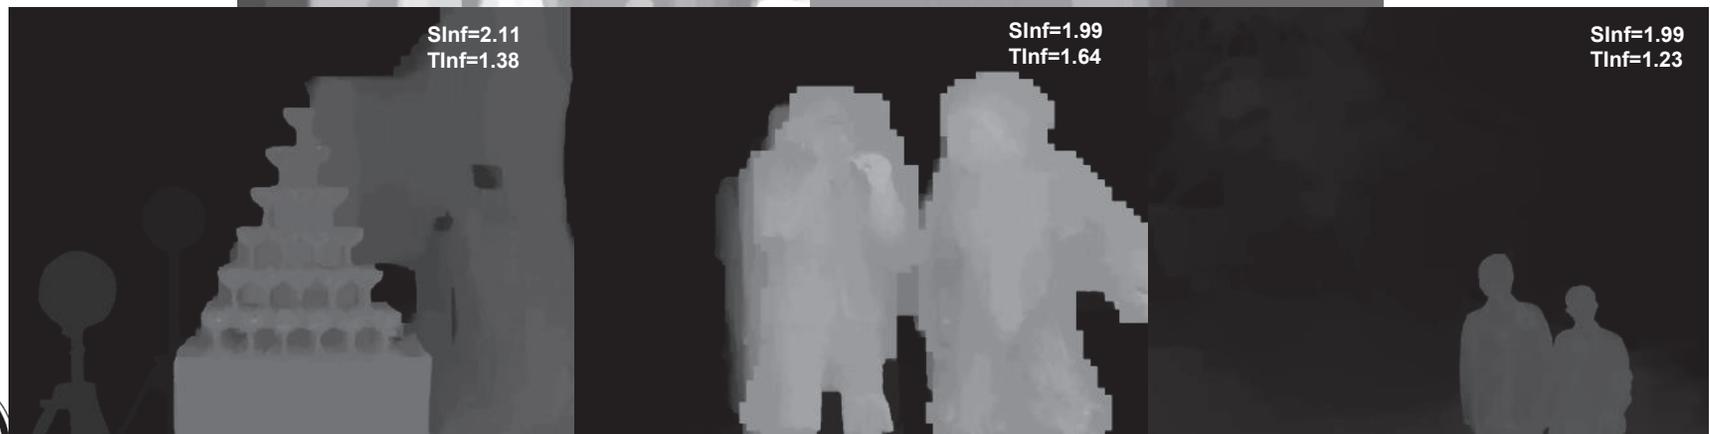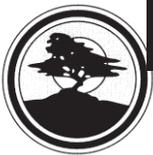

# VDM versus SSIM and PSNR

## Balloons

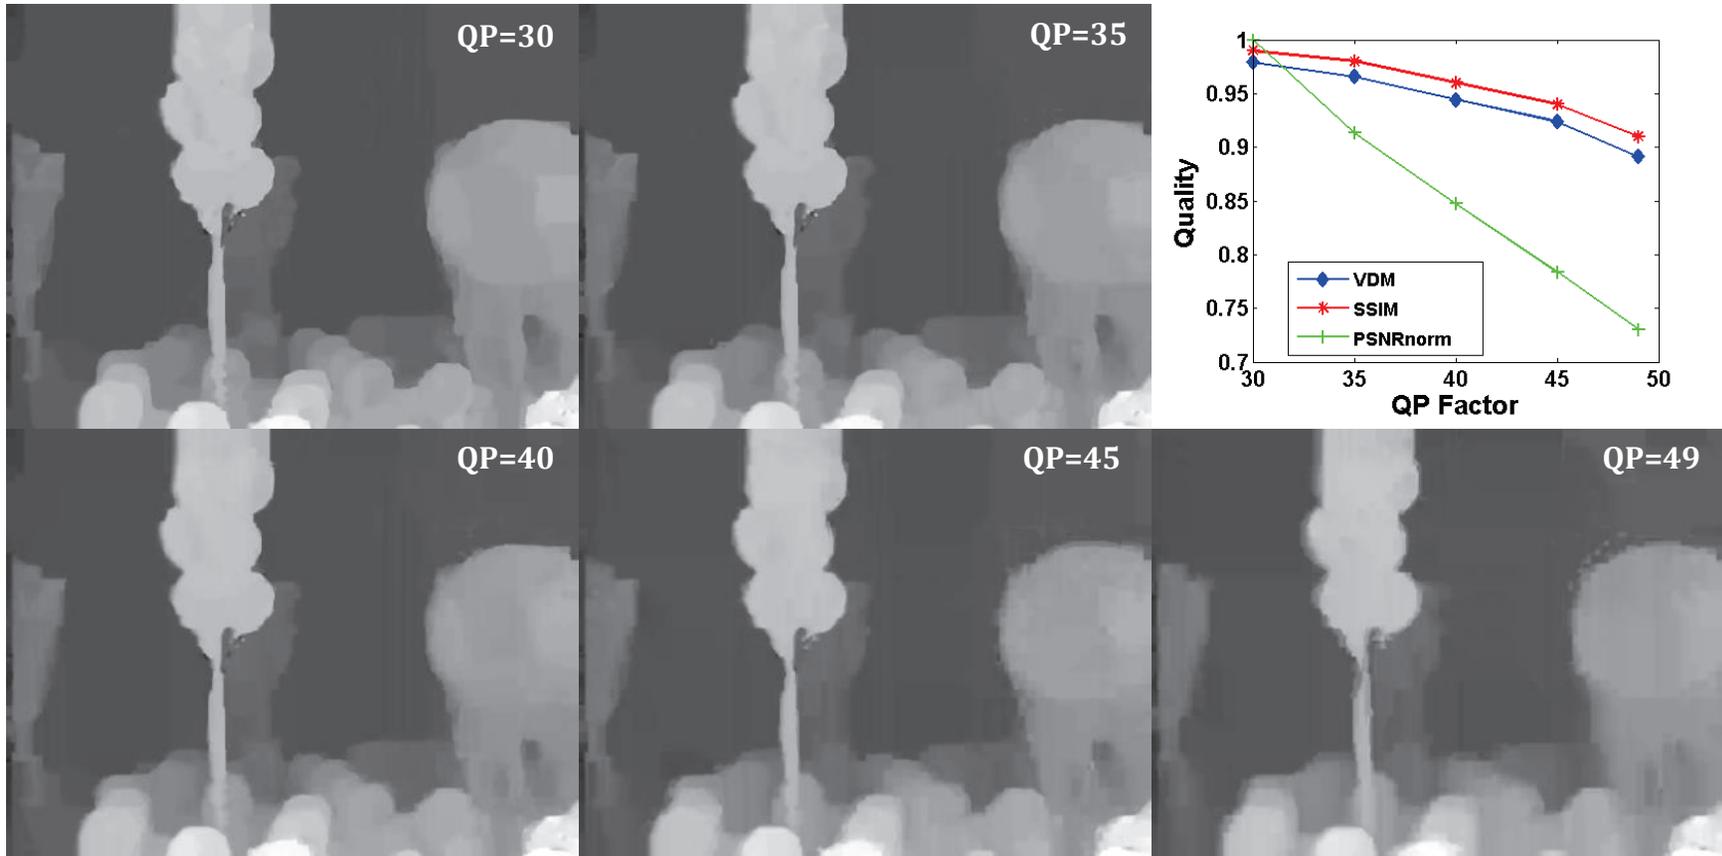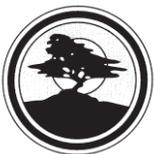

# VDM versus SSIM and PSNR

## Champagne Tower

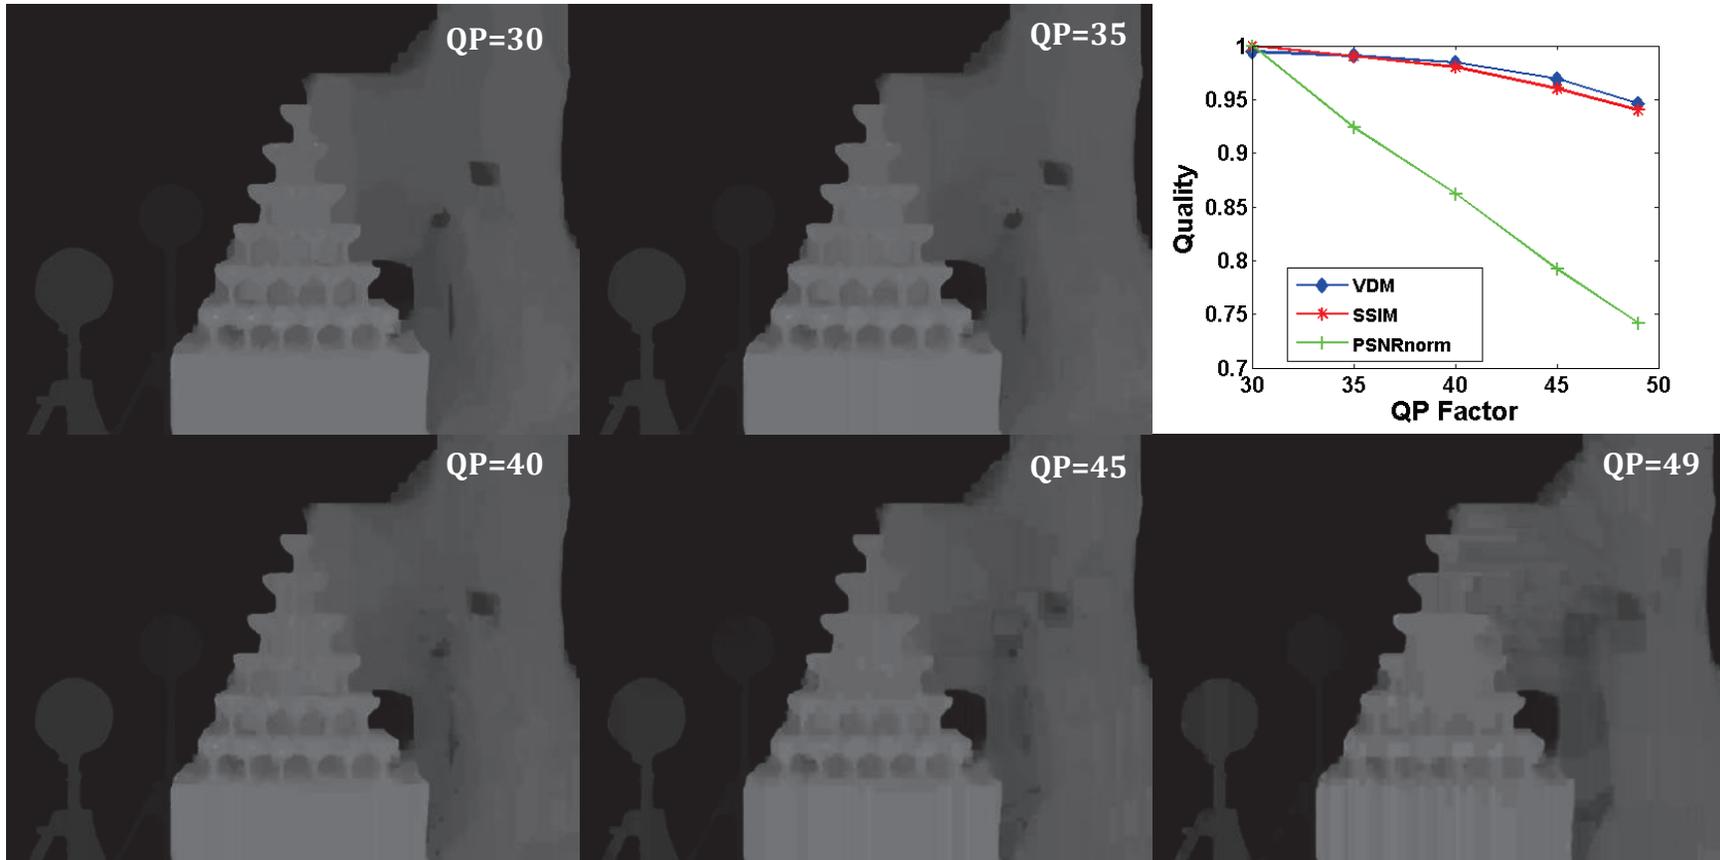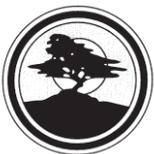

# VDM versus SSIM and PSNR

Kendo

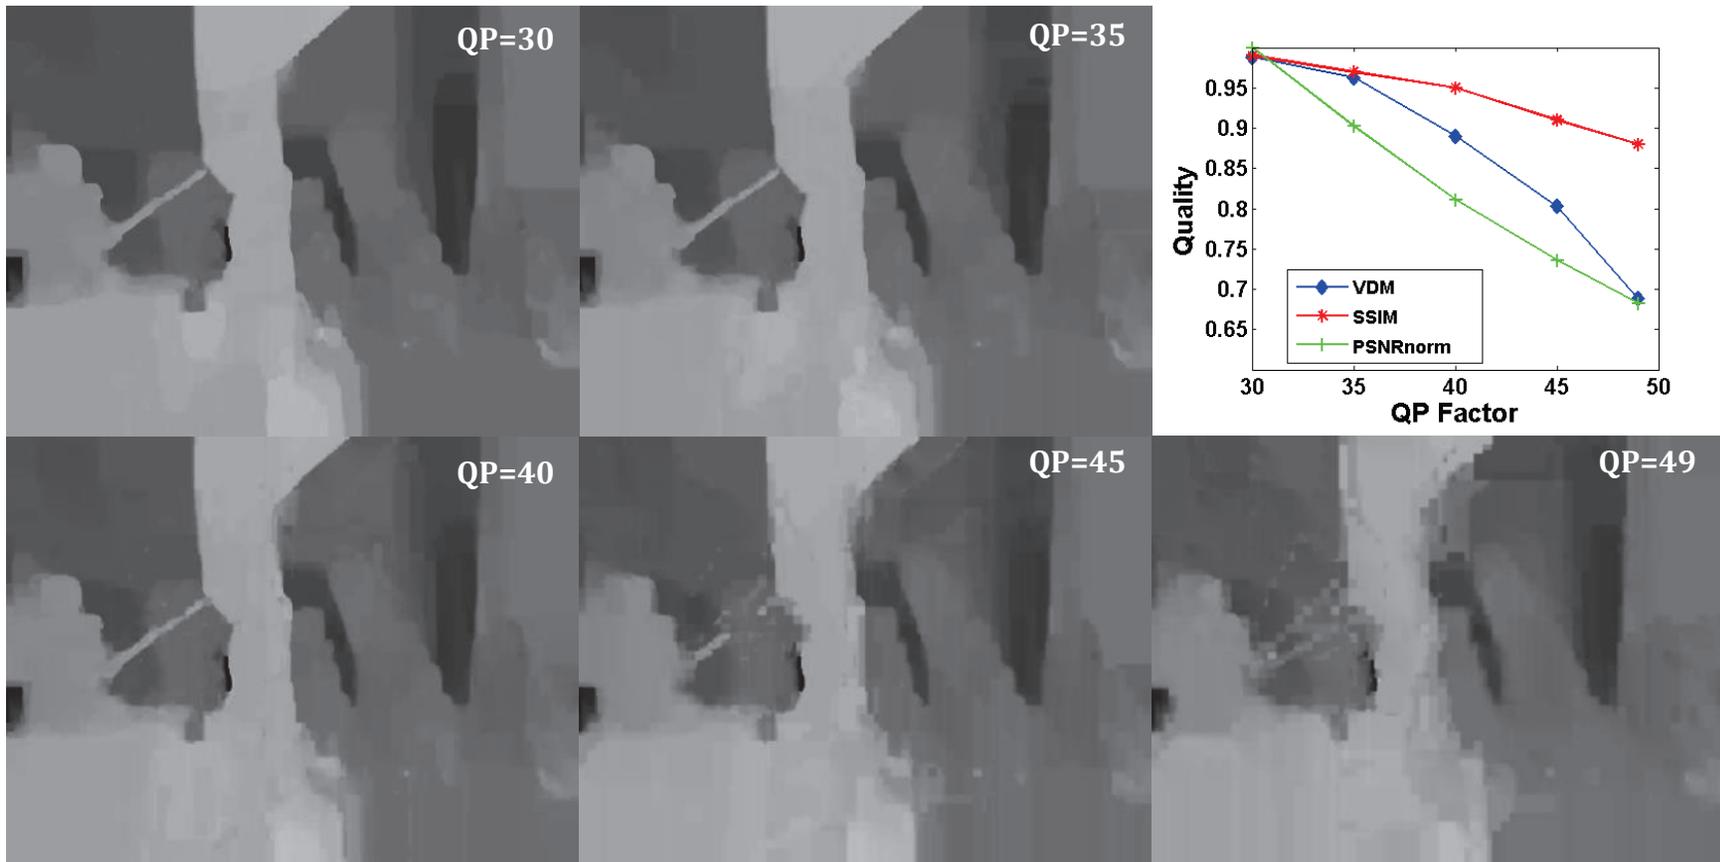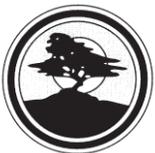

# VDM versus SSIM and PSNR

## Lovebirds

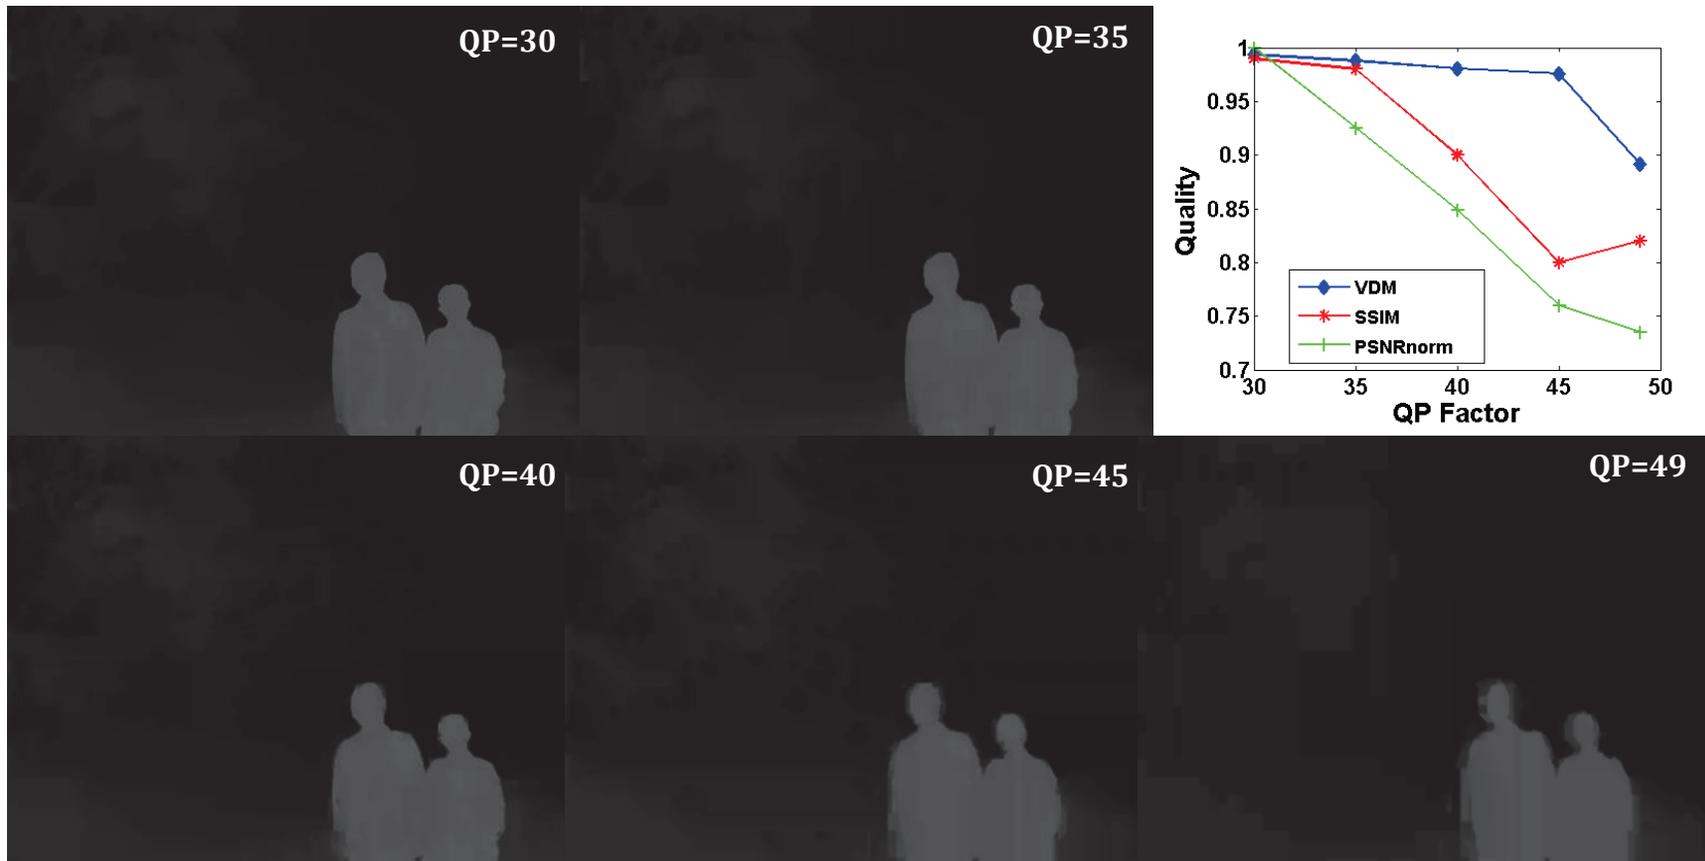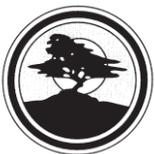

# VDM versus SSIM and PSNR

## Pantomime

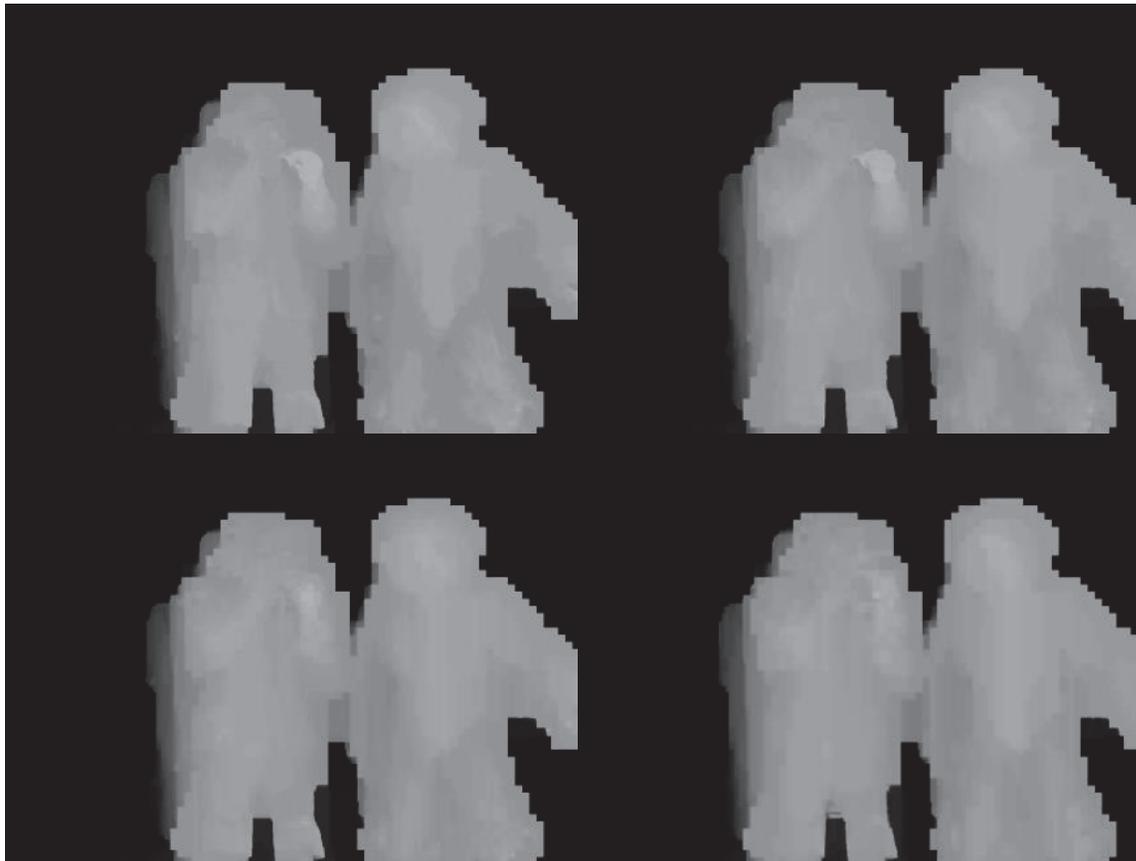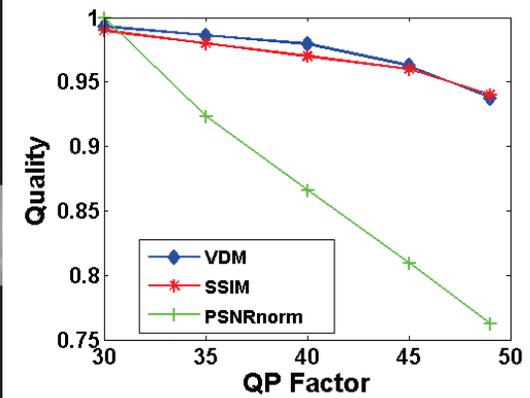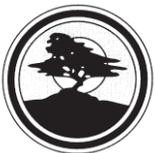

# Encoding Mode Selection

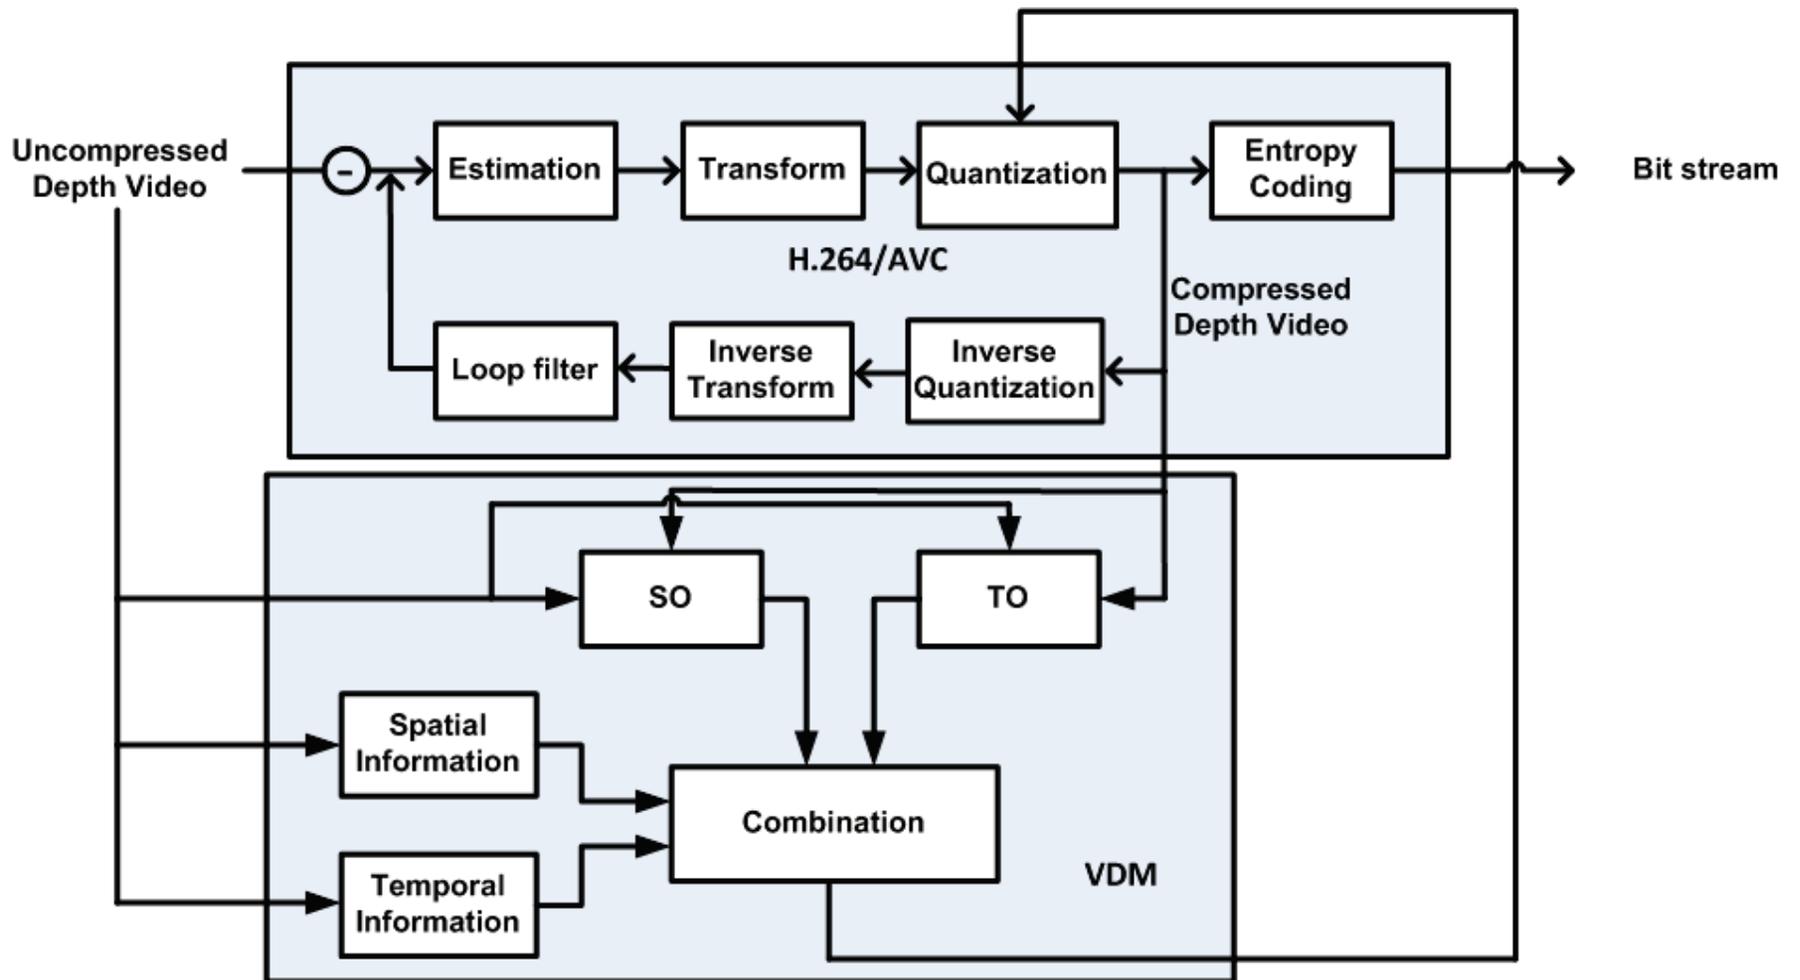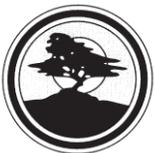

# Rate Distortion Analysis

## Balloons

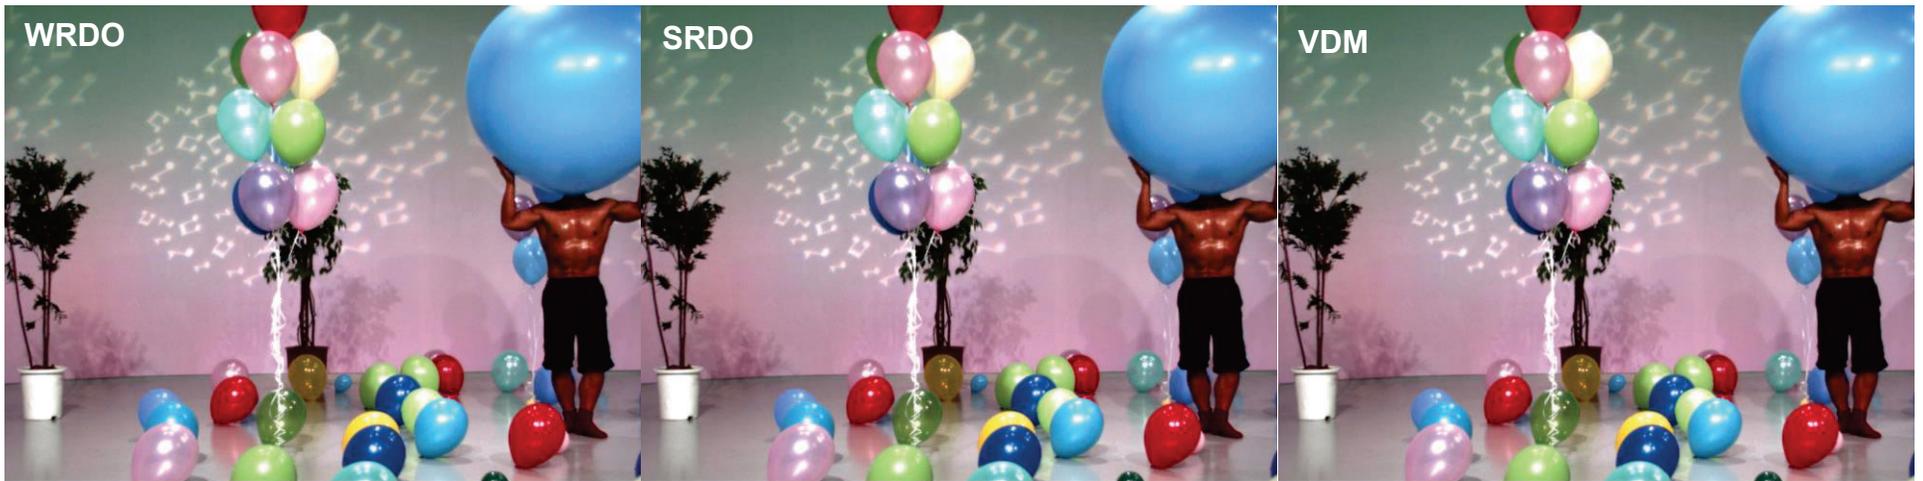

| BALLOONS | Without RDO | Standard RDO | VDM based RDO |
|----------|-------------|--------------|---------------|
| Bitrate  | 93.58       | 48.79        | 42.53         |
| PSNR     | 36.08       | 33.51        | 32.49         |
| SSIM     | 0.96        | 0.94         | 0.93          |

**WRDO:** Synthesized Video without Rate Distortion Optimization

**SRDO:** Synthesized Video with Standard Rate Distortion Optimization

**VDM:** Synthesized Video with VDM-based Rate Distortion Optimization

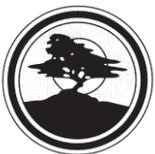

# Rate Distortion Analysis Champagne Tower

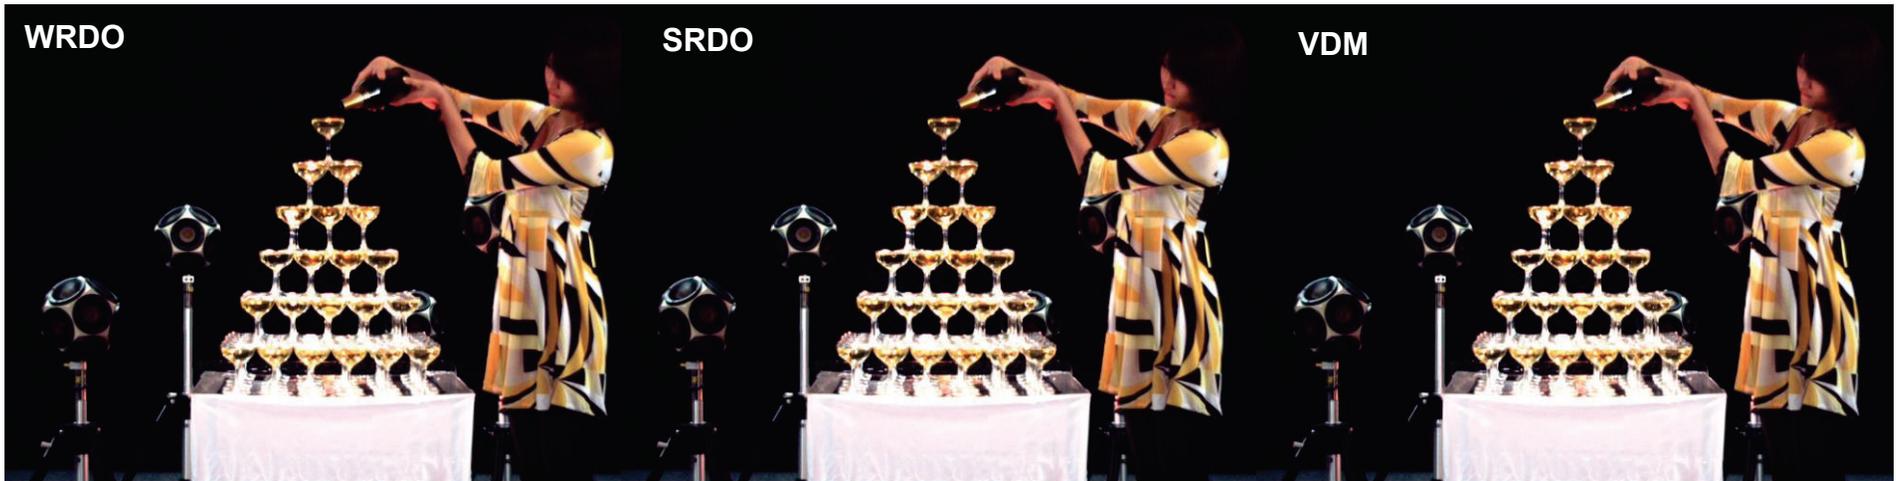

| CHAMPAGNE<br>TOWER | Without<br>RDO | Standard<br>RDO | VDM based<br>RDO |
|--------------------|----------------|-----------------|------------------|
| Bitrate            | 56.58          | 50.45           | 26.45            |
| PSNR               | 39.73          | 38.78           | 35.45            |
| SSIM               | 0.98           | 0.98            | 0.95             |

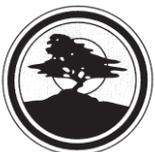

# Rate Distortion Analysis

## Kendo

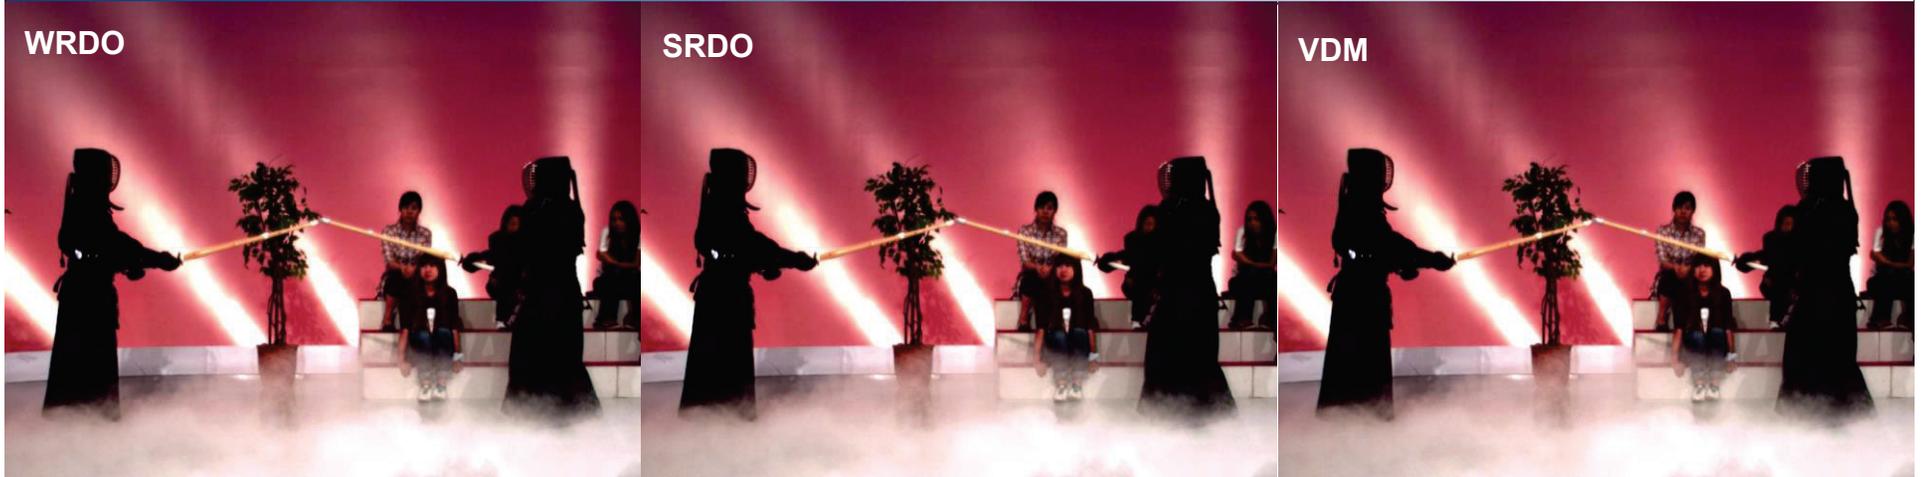

| KENDO   | Without RDO | Standard RDO | VDM based RDO |
|---------|-------------|--------------|---------------|
| Bitrate | 153.84      | 57.83        | 67.76         |
| PSNR    | 35.11       | 30.63        | 30.96         |
| SSIM    | 0.95        | 0.89         | 0.90          |

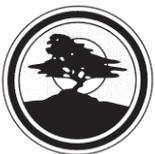

# Rate Distortion Analysis

## Lovebirds

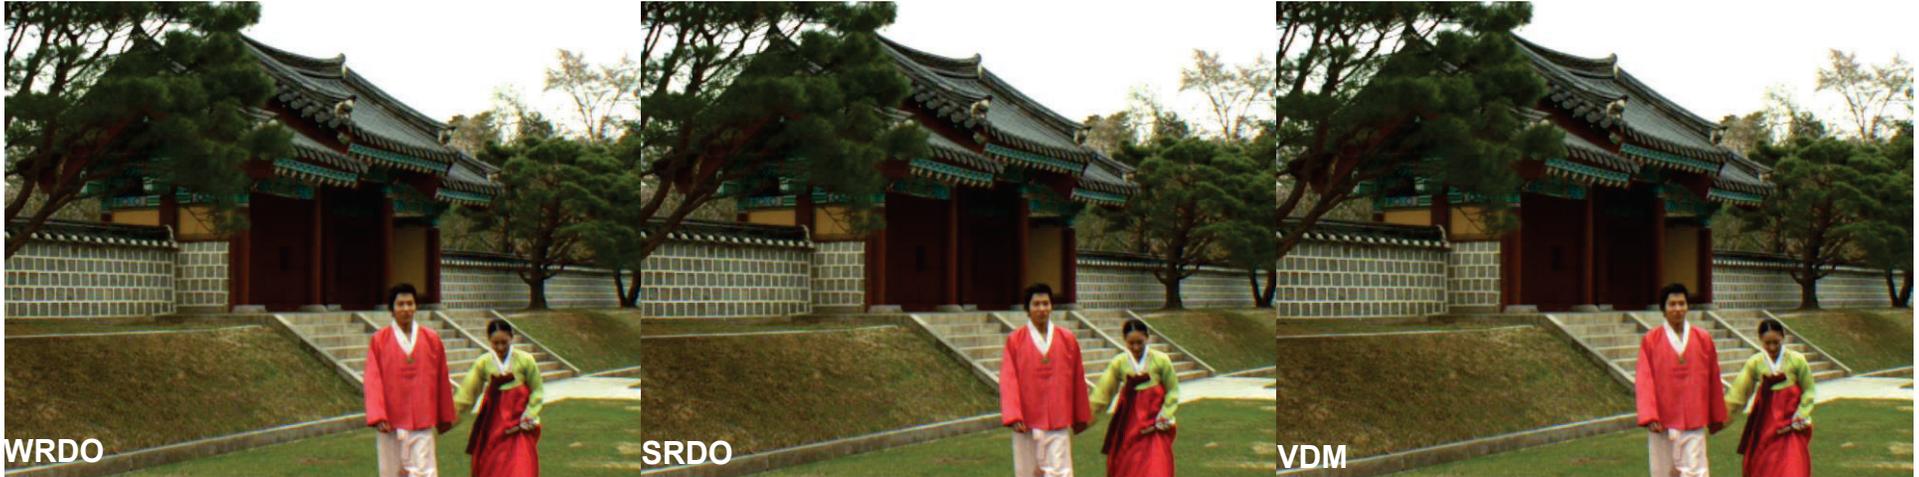

| LOVEBIRDS | Without RDO | Standard RDO | VDM based RDO |
|-----------|-------------|--------------|---------------|
| Bitrate   | 37.66       | 49.55        | 19.47         |
| PSNR      | 39.56       | 41.40        | 34.92         |
| SSIM      | 0.90        | 0.97         | 0.81          |

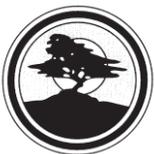

# Rate Distortion Analysis

## Pantomime

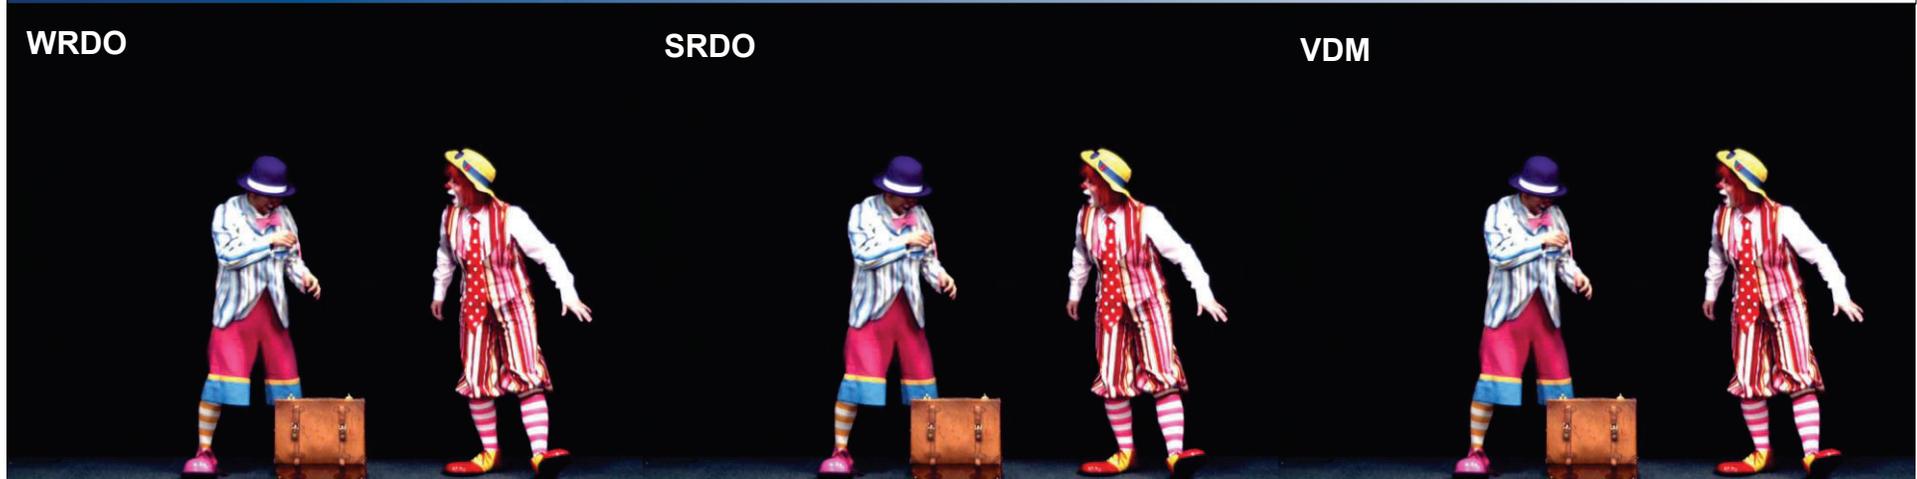

| PANTOMIME | Without RDO | Standard RDO | VDM based RDO |
|-----------|-------------|--------------|---------------|
| Bitrate   | 71.81       | 48.86        | 38.75         |
| PSNR      | 39.37       | 36.70        | 35.90         |
| SSIM      | 0.97        | 0.95         | 0.95          |

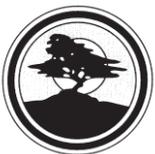

# Conclusion

## Bit rate (kbits/sec)

| Depth Sequences | WRDO         | SRDO         | VDM          |
|-----------------|--------------|--------------|--------------|
| Balloons        | 93.58        | 48.79        | 42.53        |
| Champagne       | 56.58        | 50.45        | 26.45        |
| Kendo           | 153.84       | 57.83        | 67.76        |
| Lovebird        | 37.66        | 49.55        | 19.47        |
| Pantomime       | 71.81        | 48.86        | 38.75        |
| <b>AVERAGE</b>  | <b>82.69</b> | <b>54.10</b> | <b>38.99</b> |

## PSNR (dB)

## SSIM

| Depth Sequences | PSNR (dB)    |              |              | SSIM        |             |             |
|-----------------|--------------|--------------|--------------|-------------|-------------|-------------|
|                 | WRDO         | SRDO         | VDM          | WRDO        | SRDO        | VDM         |
| Balloons        | 36.08        | 33.51        | 32.49        | 0.96        | 0.94        | 0.93        |
| Champagne       | 39.73        | 38.78        | 35.45        | 0.98        | 0.98        | 0.95        |
| Kendo           | 35.11        | 30.63        | 30.96        | 0.95        | 0.89        | 0.90        |
| Lovebird        | 39.56        | 41.40        | 34.92        | 0.90        | 0.97        | 0.81        |
| Pantomime       | 39.37        | 36.70        | 35.90        | 0.97        | 0.95        | 0.95        |
| <b>AVERAGE</b>  | <b>37.97</b> | <b>36.20</b> | <b>33.94</b> | <b>0.95</b> | <b>0.95</b> | <b>0.91</b> |

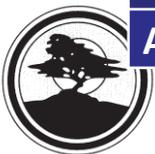

Supplement: Supplementary file 1 [file Temel2013_Asilomar.pdf]
